# Supplementary material for: Anisotropic Magnetodielectric Coupling in Layered Antiferromagnetic FePS$_3$
Source: arXiv:2208.02729 source file (2023-08-04)

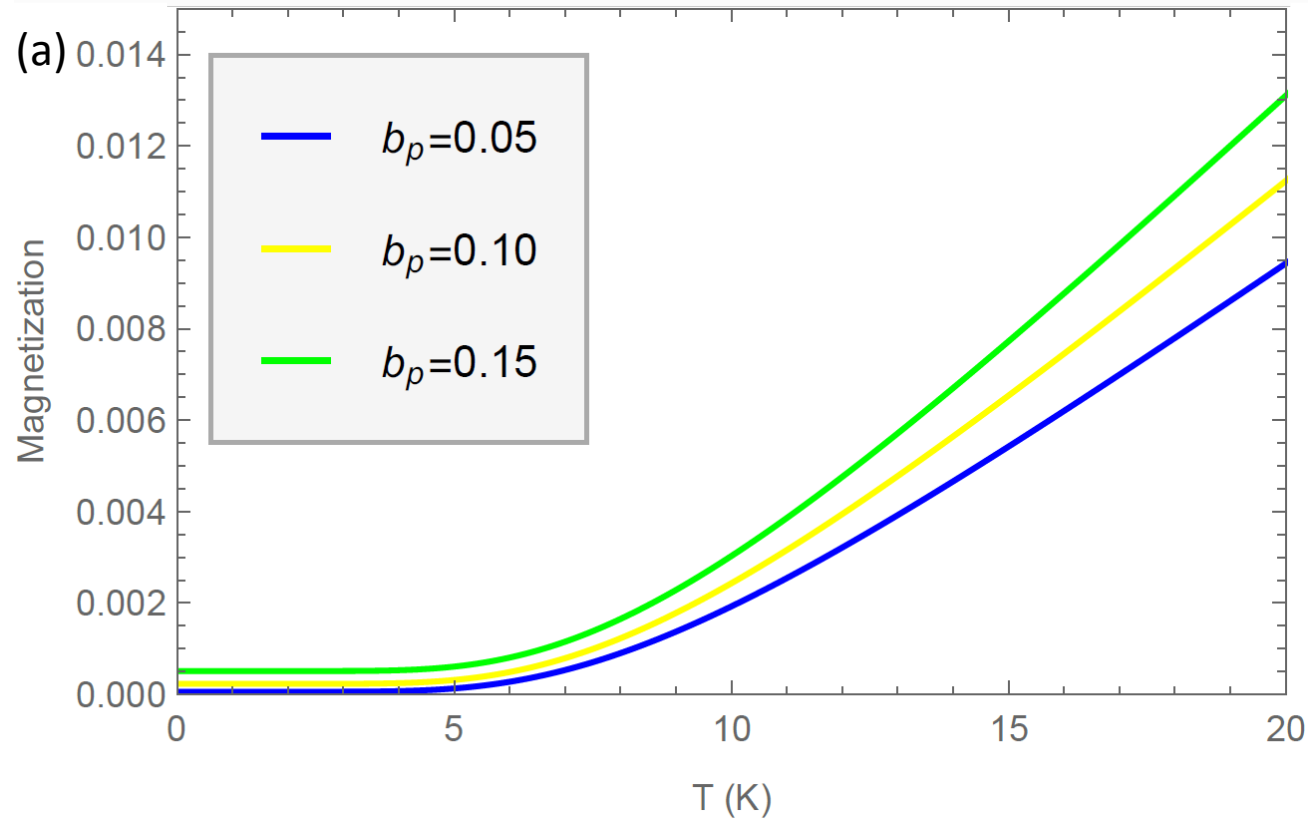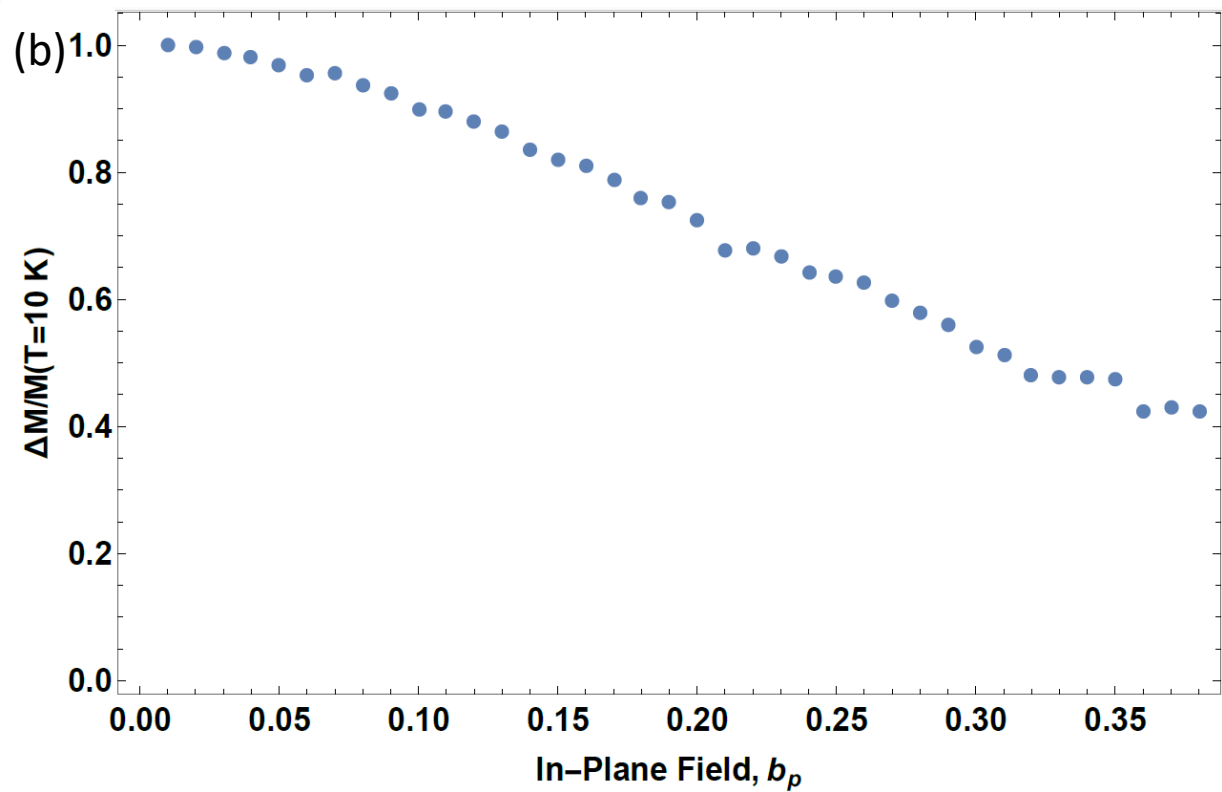

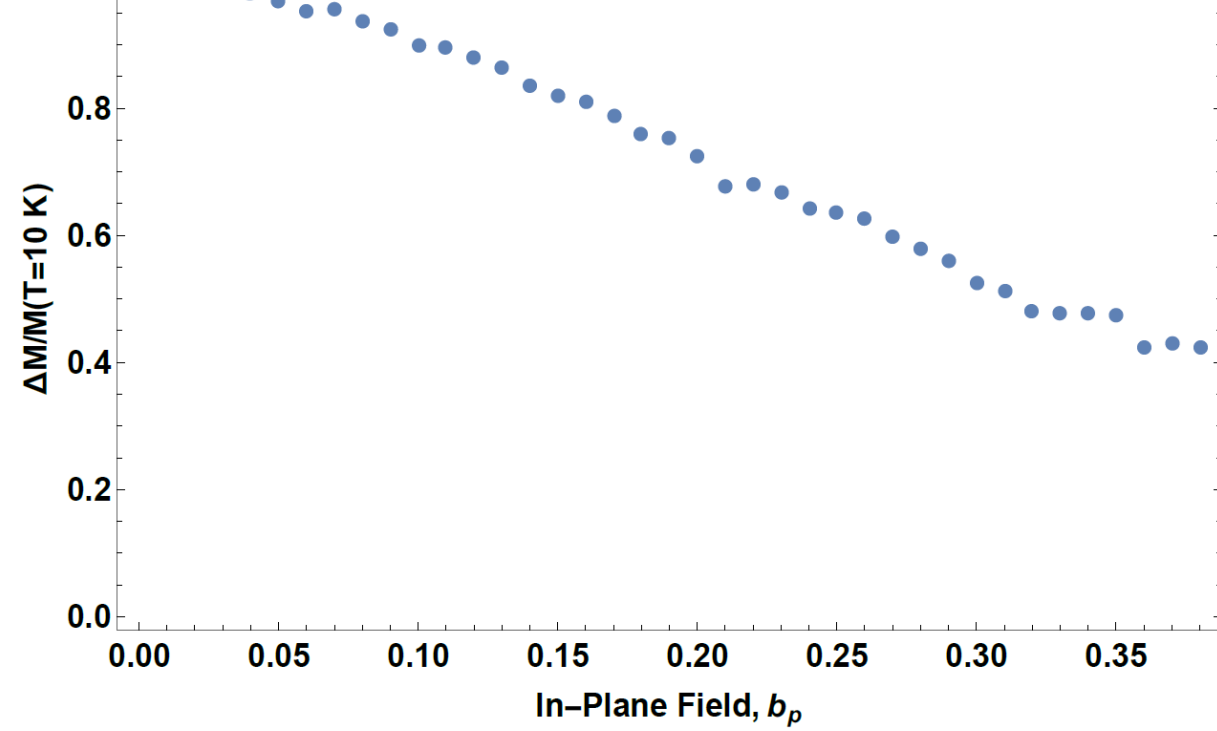

Supplement: Supplementary file 2 [file som_theory2.pdf]
